# Supplementary material for: On the Programmatic Generation of Reproducible Documents
Source: arXiv:2007.12631 source file (2020-06-23)
Supplement: Supplementary file 2 [file RJwrapper.pdf]

# Programmatic Generation of R Markdown Documents with `listdown`

by Michael Kane

**Abstract** An abstract of less than 150 words.

## Background and concepts

R Markdown documents support the construction of reproducible documents by allowing authors to insert R code for data processing, exploration, analysis, table-making, and visualization directly into structured, prose documents. In the context of this document, we will refer to the R code in these documents as *computational components* since they are generated by computational means (namely the R interpreter). The prose in these documents will be referred to as *narrative components*. They may serve to help a reader understand the background, goal, theme, and results of the paper as well as contextualizing the computational components.

R Markdown (Baumer et al., 2014) integrates the process of integrating the computational and narrative components of a document. By itself this is not novel. It was identified as “Literate Programming” by Knuth (1984) and software tools, like Sweave (Leisch, 2002) have supported this functionality for almost two decades. R Markdown’s popularity has likely been driven by two factors. The first is the relative ease with which these documents can be constructed. While it is more expressive,  $\text{\LaTeX}$  is relatively technical and requires an investment in time to become proficient. By contrast R Markdown documents are easier to create and format and, when the document is used to create  $\text{\LaTeX}$  formatting can be passed through to the underlying .tex file. The second factor driving adoption is likely its support for creating *modifiable* documents, Microsoft Word in particular. Researchers and analysts, especially those creating applied statistical analyses, often collaborate with domain experts with less technical knowledge. In these cases, the analyst focuses on creating the computational components and narrative components related to results and interpretation. After this initial document is created, the domain expert is free to develop narrative components directly in the document without needing to go through the analyst.

Since computational components are, by definition, computationally derived objects and R Markdown is a well-defined standard it is possible to programmatically create R Markdown documents with computational components. This is the focus of this paper. However, before proceeding down this avenue, we would like to highlight two fundamental limitations to automated R Markdown document construction. First and foremost, without narrative components a document has no context. Quantitative analyses require research questions, hypotheses, reviews, interpretations, and conclusions. Computational components are necessary but not sufficient for constructing an analysis. Second, it is not possible to construct computational components for an arbitrary analyses. Analyses themselves have context and are built with a set of assumptions and goals. Computational components are constructed for a narrow class of problems.

However, this is not to say the programmatic creation of R Markdown documents is unwarranted or not useful. In fact, it has at least two appealing characteristics. The first is that it allows us to distinguish the presentation of analytical results from other steps in a data science or data processing pipeline. These other steps including cleaning and analysis often require their own environment and configuration with requirements very different than the computational needs of creating a presentation. By separating these components each can be developed independently. At the same time, by specifying that the output of those objects are organized hierarchically, we are essentially creating a contract by which processed data can be passed to the presentation as well as providing a way to organize the results. The second reason for programmatic creation of R Markdown documents is convenience. In collaborative environments, especially in the early stages, large numbers of graphs and tables are generated and discussed. By collecting these artifacts hierarchically as a list, they can be quickly iterated upon and restructured to more clearly present the data without needing to spend time on the creation of the presentation document.

The `listdown` package provides functions to programmatically create R Markdown files from named lists. It is intended for data analysis pipelines where the presentation of the results is separated from their creation. For this use case, a data processing (or analysis) is performed and the results are provided in a single named list, organized hierarchically. With the list and a `listdown` object a `workflowr` (Blischak et al., 2019), pdf, word, or html page. List element names denote sections, subsections, subsubsection, etc. and the list elements contain the data structure to be presented including graphs and tables. The goal of the package is not to provide a finished, readable document. It

is to provide a document with all tables and visualization that will appear (*computational* components). This serves as a starting point from which a user can organize outputs, describe a study, discuss results, and provide conclusions (*narrative* components).

**listdown** provides a reproducible means for producing a document with specified computational components. It is most compatible with data analysis pipelines where the data format is fixed but the analyses are either being updated, which may affect narrative components including the result discussion and conclusion, or where the experiment is different, which affects all narrative components. If the narrative components are not changing with the data being pushed through your analysis pipeline, then you may be better off writing the R Markdown code manually.

One area where we have found **listdown** is particularly useful is in the reporting and research of clinical trial data. These collaborations tend to be between (bio)statisticians and clinicians either analyzing past trial data to formulate a new trial or in trial monitoring where trial telemetry (enrollment, responses, etc.) is reported and initial analyses are conveyed to a clinician. The associated presentations require very little context - clinicians often have a better understanding of the data collected than the statistician - often eliminating the need for narrative components. At the same time, a large number of hierarchical, heterogeneous artifacts (tables and multiple types of plots) need to be conveyed thereby making the manual creation of R Markdown documents inconvenient.

Furthermore, data processing can be fixed across trials. This is especially true in the initial stages, which focus on patient demographics and enrollment. This has made it convenient for our group to quickly generate standardize and complete reports for multiple trials concurrently. To date, we have used **listdown** to report on five clinical trials, with another two currently in process. Results are disseminated using the **workflowr** package, usually with nine tabs conveying aspects of the data from collection through several different analyses, and each tab containing approximately five to thirty tables, plots, or other artifacts including **trelliscopejs** (Hafen and Schloerke, 2020) environments which may hold hundreds of graphs. By generating many presentation artifacts we are able to address data-drive questions and issues during collaborative sessions and by carefully structuring these elements we allowing all members to participate in the process.

The **listdown** package itself is relatively simple with 6 distinct methods that can be easily incorporated into existing analysis pipelines for automatically creating documents that can be used for data exploration and reviewing analysis results as well as a starting point for a more formal write up. These methods include:

- **as\_ld\_yaml()** - turn a computational component list into YAML with class information
- **ld\_cc\_dendro()** - create a dendrogram from a list of computational components
- **ld\_chunk\_opts()** - apply chunk options to a presentation object
- **ld\_ioslides\_header()** - create an ioslides presentation header
- **ld\_make\_chunks()** - write a listdown object to a string
- **ld\_rmarkdown\_header()** - create an R Markdown header
- **ld\_workflowr\_header()** - create a workflowr header
- **listdown()** - create a listdown object to create an R Markdown document

The rest of this paper is structured as follow. The next section goes over basic usage and commentary. This section is meant to convey the basic approach used by the package and shows how to describe an output document using **listdown**, create a document, and change how the presentation of computational components can be specialized using **listdown** decorators. With the user accustomed to the package's basic usage, section 3 describes the design of the package. Section 4 goes over advanced usage of the package including adding initialization code to and outputted document as well as how to control chunk-level options. Section 5 concludes the paper with a few final remarks.

## Basic usage and overview

Suppose we have just completed an analysis and have collected all of the results into a list where the list elements are roughly in the order we would like to present them in a document. It may be noted that this is not always how computational components derived from data analyses are collated. Often individual components are stored in multiple locations on a single machine or across machines. However, it is important to realize that even for analyses on large-scale data, the digital artifacts to be presented are relatively small. Centralizing them makes it easier to access them, since they don't need to be found in multiple locations. Also, storing them as a list provides a hierarchical structure that translates directly to a document as we will see below.

As a first example, we will consider the a list of visualizations from the `anscombe` data set. The list is composed of four **ggplot2** (Wickham, 2016) elements (named Linear, Non Linear, Outlier Vertical, and Outlier Horizontal) each containing a scatter plot from the famous Anscombe Quartet - made available in the **datasets** package (R Core Team, 2012). From the `computational_components` list, we would like to create a document with four sections with names corresponding to the list names, each containing their respective visualizations.

```
# Use ggplot2 to create the visualizations.
library(ggplot2)

# Load the Anscombe Quartet.
data(anscombe)

# Create the ggplot objects to display.
computational_components <- list(
  Linear = ggplot(anscombe, aes(x = x1, y = y1)) + geom_point(),
  `Non Linear` = ggplot(anscombe, aes(x = x2, y = y2)) + geom_point(),
  `Outlier Vertical` = ggplot(anscombe, aes(x = x3, y = y3)) + geom_point(),
  `Outlier Horizontal` = ggplot(anscombe, aes(x = x4, y = y4)) + geom_point())

# Save the file to disk to be read by the output R Markdown document.
saveRDS(computational_components, "comp-comp.rds")
```

### Creating a document with listdown

Creating a document from the `computational_components` will require two steps. First, we will create a `listdown` object that specifies how the `computational_components` object will be loaded into the document, which libraries and code needs to be included, and how the list elements will be presented in the output R markdown document.

```
library(listdown)

ld <- listdown(load_cc_expr = readRDS("comp-comp.rds"),
               package = "ggplot2")
```

The `ld` object, along with the computational components in the `comp-comp.rds` file are sufficient to create the sections, subsections, and R chunks of a document. The only other thing requires to create the document is the header. The `listdown` package currently supports regular R Markdown and **workflowr** as `yaml` objects from the **yaml** package (Stephens et al., 2020). These objects are stored as named lists in R and are easily modified to accomodate document parameters. A complete document can then be written to the console using the code shown below. It could easily be written to a file for rendering using the `writelnLines()` as in the following example.

```
doc <- c(
  as.character(
    ld_rmarkdown_header("Anscombe's Quartet",
                        author = "Francis Anscombe",
                        date = "1973")),
  ld_make_chunks(ld))

cat(paste(doc, collapse = "\n"))

#> ---
#> title: Anscombe's Quartet
#> author: Francis Anscombe
#> date: '1973'
#> output: html_document
#> ---
#> 
#> ```{r}
#> library(ggplot2)
#> 
#> cc_list <- readRDS("comp-comp.rds")
#> ```
#>
```

```

#> # Linear
#>
#> ```{r}
#> cc_list$Linear
#> ```
#>
#> # Non Linear
#>
#> ```{r}
#> cc_list$`Non Linear`
#> ```
#>
#> # Outlier Vertical
#>
#> ```{r}
#> cc_list$`Outlier Vertical`
#> ```
#>
#> # Outlier Horizontal
#>
#> ```{r}
#> cc_list$`Outlier Horizontal`
#> ```

```

The `listdown()` function provides *document-wide* R chunk options for displaying computational components. The chunk options are exactly the same as those in the R markdown document and can be used to tailor the default presentation for a variety of needs. The complete set of options can be found in the [R Markdown Reference Guide](#). As a concrete example, the code used to create present the plots could be hidden in the output document using the following code.

```

ld <- listdown(load_cc_expr = readRDS("comp-comp.rds"),
               package = "ggplot2",
               echo = FALSE)

cat(paste(ld_make_chunks(ld)[1:7], collapse = "\n"))

#>
#> ```{r echo=FALSE}
#> library(ggplot2)
#>
#> cc_list <- readRDS("comp-comp.rds")
#> ```

```

## Decorators

The first example is simple in part because the ggplot objects both contain the data we want to display and, at the same time, provide the mechanism for presenting them - rendering them in a graph. However, this is not always the case. The objects being stored in the list of computational components may not translate directly to the presentation in a document. In these cases, a function is needed that takes the list component and returns an object to be displayed. For example, suppose that, along with showing graphs from the Anscombe Quartet, we would like to include the data themselves. We could add the data to the `computational_components` list and then create the document with:

```

computational_components$Data <- anscombe
saveRDS(computational_components, "comp-comp.rds")
cat(paste(ld_make_chunks(ld)[32:36], collapse = "\n"))

#> # Data
#>
#> ```{r echo=FALSE}
#> cc_list$Data
#> ```

```

In this case, the **listdown** package will show the entire data set as is the default specified. However, suppose we do not want to show the entire data set in the document. This is common, especially when

the data set is large and requires too much vertical space in the outputted document resulting in too much or irrelevant data being shown. Instead, we would like to output to an html document where the data is shown in a datatable thereby controlling the amount of real-estate needed to present the data and, at the same time, providing the user with interactivity to sort and search the data set.

In **listdown**, a function or method that implements the presentation of a computational component is referred to as a *decorator* since it follows the classic decorator pattern described in [Gamma et al. \(1995\)](#). A decorator takes the element that will be presented as an argument and returns an object for presentation in the output directory. A decorator is specified using the `decorator` parameter of the `listdown()` function using a named list where the name corresponds to the type and the element correspond to the function or method that will decorate an object of that type. For example, the `anscombe` data set can be decorated with the `DT::datatable()` function ([Xie et al., 2020](#)) as:

```
ld <- listdown(load_cc_expr = readRDS("comp-comp.rds"),
               package = c("ggplot2", "DT"),
               decorator = list(data.frame = datatable))
cat(paste(ld_make_chunks(ld)[33:37], collapse = "\n"))

#> # Data
#>
#> ```{r}
#> datatable(cc_list$Data)
#> ```
```

List names in the decorator argument provide a key to which a function or method is mapped. The underlying decorator resolution is implemented for a given computational component by going through decorator names sequentially to see if the component inherits from the name using the `inherits()` function. The function or method is selected from the corresponding name which the element first inherits from. This means that when customizing the presentation of objects that inherit from a common class, the more abstract classes should appear at the end of the list. This will ensure that specialized classes will be encountered first in the resolution process. It should be noted that an object's type is first checked against the decorator name list and then checked to see if it is a list. This allows a user to both decorate a list and retain "list" in its class attributes.

A separate argument, `default_decorator`, allows the user to specify the default decorator for an object whose type does not appear in the decorator list. This allows the user to specify any class name for the decorator and avoids a potential type name collision with a default decorator whose name is determined by convention. By default, this argument is set to `identity` but it can be used to not display a computational component by default if the argument is set to `NULL`.

## Design

A **listdown** object specifies the location of a list of computational components and options for presenting those components in an R Markdown document. The list is a hierarchical data structure that also provides the structure of the outputted document. A corresponding document has two sections "Iris" and "Sepal.Length". The latter has three subsections "Sepal.Width", "Petal.Length", and "Colored". The "Colored" subsection has two sub-subsections, "Sepal.Width" and "Petal.Length". The structure can be seen using the `ld_cc_dendro()` function.

```
# Create a more hierarchical list of computational components.
comp_comp2 <- list(
  Iris = iris,
  Sepal.Length = list(
    Sepal.Width = ggplot(iris, aes(x = Sepal.Length, y = Sepal.Width)) + geom_point(),
    Petal.Length = ggplot(iris, aes(x = Sepal.Length, y = Sepal.Width)) + geom_point(),
    Colored = list(
      Sepal.Width = ggplot(iris, aes(x = Sepal.Length, y = Sepal.Width, color = Species)) +
        geom_point(),
      Petal.Length = ggplot(iris, aes(x = Sepal.Length, y = Petal.Length, color = Species)) +
        geom_point()
    )
  )

# Create the dendrogram.
ld_cc_dendro(comp_comp2)

#>
#> comp_comp2
```

```

#> |-- Iris
#> | o-- object of type(s):data.frame
#> o-- Sepal.Length
#> |-- Sepal.Width
#> | o-- object of type(s):gg ggplot
#> |-- Petal.Length
#> | o-- object of type(s):gg ggplot
#> o-- Colored
#> |-- Sepal.Width
#> | o-- object of type(s):gg ggplot
#> o-- Petal.Length
#> o-- object of type(s):gg ggplot
#>

```

Both the `ld_cc_dendro()` and `ld_make_chunks()` functions work by recursively descending the computational components list depth-first. If the list containing an element has a name, it is written to the output as a section, subsection, subsubsection, etc. to a return string. If the visited list element is itself a list, then the same procedure is called on the child list through a recursive call. If the element is not a list, then it is outputted inside an R Markdown chunk in the return string using the appropriate decorator.

## R code chunk customization

Along with the basic usage, the **listdown** package supports two other capabilities to further customize the presentation. The first is where custom code is required either to modify decorators or even define a decorator. In this case, we would add a small portion of code, immediately after loading required libraries. In the second case, rather than changing the R code inside of a chunk, we would like to change the options for an individual chunk. Both of these features are supported in the package and are presented below.

### Initialization code

```

saveRDS(comp_comp2, "comp-comp2.rds")
ld <- listdown(load_cc_expr = readRDS("comp-comp2.rds"),
               package = c("ggplot2", "DT", "purrr"),
               decorator = list(ggplot = identity,
                                data.frame = datatable),
               init_expr = {
                 datatable <- partial(datatable,
                                       options = list(dom = 't'))
               },
               echo = FALSE)

cat(paste(ld_make_chunks(ld)[1:13], collapse = "\n"))

#>
#> ```{r echo=FALSE}
#> library(ggplot2)
#> library(DT)
#> library(purrr)
#>
#> cc_list <- readRDS("comp-comp2.rds")
#> ```
#>
#> ```{r echo=FALSE}
#>
#> datatable <- partial(datatable, options = list(dom = "t"))
#> ```

```

### Controlling chunk-level options

Along with providing document-wide chunk options, it is also possible to control individual chunk options

```

comp_comp2$Iris <- ld_chunk_opts(comp_comp2$Iris, echo = TRUE)
saveRDS(comp_comp2, "comp-comp2.rds")
cat(paste(ld_make_chunks(ld)[1:19], collapse = "\n"))

#>
#> ```{r echo=FALSE}
#> library(ggplot2)
#> library(DT)
#> library(purrr)
#>
#> cc_list <- readRDS("comp-comp2.rds")
#> ```
#>
#> ```{r echo=FALSE}
#>
#> datatable <- partial(datatable, options = list(dom = "t"))
#> ```
#>
#> # Iris
#>
#> ```{r echo = TRUE}
#> datatable(cc_list$Iris)
#> ```

```

## A simple example: Reporting on the gtsummary::trial dataset

```

library(gtsummary)
library(dplyr)
library(glue)
library(survival)
library(survminer)
library(rmarkdown)

# Function to create the computational components.
make_surv_cc <- function(trial, treat, surv_cond_chars) {
  # Create Table 1 by treatment
  table_1 <- trial %>%
    tbl_summary(by = all_of(treat)) %>%
    gtsummary::as_flextable()

  # Create survival plots base on survival characteristics
  scs <- lapply(c("1", surv_cond_chars),
    function(sc) {
      glue("Surv(ttdeath, death) ~ {treat} + {sc}") %>%
        as.formula() %>%
        surv_fit(trial) %>%
        ggsurvplot()
    })
  names(scs) <- c("Overall", tools::toTitleCase(surv_cond_chars))
  list(`Table 1` = table_1, `Survival Plots` = scs)
}

# Create the computational components and write to surv-cc.rds.
make_surv_cc(trial, treat = "trt",
  surv_cond_chars = c("stage", "grade")) %>%
  saveRDS("surv-cc.rds")

# Create the listdown object with appropriate dependencies
# and presentation parameters.
ld_surv <- listdown(load_cc_expr = readRDS("surv-cc.rds"),
  package = c("gtsummary", "survminer"),
  decorator = list(ggsurvplot = identity,
    tbl_summary = identity),

```

```
      echo = FALSE,
      message = FALSE,
      warning = FALSE,
      fig.width = 7,
      fig.height = 4.5)

# Write an RMarkdown header and chunks derived from the
# computational components and listdown object to trial-report.rmd.
writeLines(
  paste(c(
    as.character(ld_rmarkdown_header("Simple Trial Report")),
    ld_make_chunks(ld_surv))),
  "trial-report.rmd")

# Render the RMarkdown file to html.
render("trial-report.rmd", quiet = TRUE, pdf_document(keep_tex = TRUE))
```

## Using listdown in practice for clinical trial reporting



## Appendix 1: RMarkdown produced in the simple example

```
---
title: Simple Trial Report
output: html_document
---

\`\`\`{r echo=FALSE}
library(gtsummary)
library(survminer)

cc_list <- readRDS("surv-cc.rds")
\`\`\`

# Table 1

\`\`\`{r echo=FALSE}
cc_list$`Table 1`
\`\`\`

# Survival Plots

## Overall

\`\`\`{r echo=FALSE}
cc_list$`Survival Plots`$Overall
\`\`\`

## Stage

\`\`\`{r echo=FALSE}
cc_list$`Survival Plots`$Stage
\`\`\`

## Grade

\`\`\`{r echo=FALSE}
cc_list$`Survival Plots`$Grade
\`\`\`
```

## Appendix 2: The document produced by the simple example

### Bibliography

- B. Baumer, M. Cetinkaya-Rundel, A. Bray, L. Loi, and N. J. Horton. R markdown: Integrating a reproducible analysis tool into introductory statistics. *arXiv preprint arXiv:1402.1894*, 2014. [p1]
- J. D. Blischak, P. Carbonetto, and M. Stephens. Creating and sharing reproducible research code the workflowr way [version 1; peer review: 3 approved]. *F1000Research*, 8(1749), 2019. doi: 10.12688/f1000research.20843.1. URL <https://doi.org/10.12688/f1000research.20843.1>. [p1]
- E. Gamma, R. Helm, R. Johnson, and J. Vlissides. Design patterns: elements of reusable object-oriented software. *Addison Wesley Longman, Inc, January*, 1(5):1, 1995. [p5]
- R. Hafen and B. Schloerke. *trelliscopejs: Create Interactive Trelliscope Displays*, 2020. URL <https://CRAN.R-project.org/package=trelliscopejs>. R package version 0.2.4. [p2]
- D. E. Knuth. Literate programming. *The Computer Journal*, 27(2):97–111, 1984. [p1]
- F. Leisch. Sweave: Dynamic generation of statistical reports using literate data analysis. In *Compstat*, pages 575–580. Springer, 2002. [p1]
- R Core Team. *R: A Language and Environment for Statistical Computing*. R Foundation for Statistical Computing, Vienna, Austria, 2012. URL <http://www.R-project.org/>. ISBN 3-900051-07-0. [p3]
- J. Stephens, K. Simonov, Y. Xie, Z. Dong, H. Wickham, J. Horner, reikoch, W. Beasley, B. O'Connor, and G. R. Warnes. *yaml: Methods to Convert R Data to YAML and Back*, 2020. URL <https://CRAN.R-project.org/package=yaml>. R package version 2.2.1. [p3]
- H. Wickham. *ggplot2: Elegant Graphics for Data Analysis*. Springer-Verlag New York, 2016. ISBN 978-3-319-24277-4. URL <https://ggplot2.tidyverse.org>. [p3]
- Y. Xie, J. Cheng, and X. Tan. *DT: A Wrapper of the JavaScript Library 'DataTables'*, 2020. URL <https://CRAN.R-project.org/package=DT>. R package version 0.12. [p5]

Michael Kane  
Yale University  
60 College Street  
New Haven, CT 06510, USA  
[michael.kane@yale.edu](mailto:michael.kane@yale.edu)
