# Supplementary material for: On the Programmatic Generation of Reproducible Documents
Source: arXiv:2007.12631 source file (2020-06-23)
Supplement: Supplementary file 3 [file trial-report.tex]

% Options for packages loaded elsewhere
\PassOptionsToPackage{unicode}{hyperref}
\PassOptionsToPackage{hyphens}{url}
\documentclass[
]{article}
\usepackage{lmodern}
\usepackage{amssymb,amsmath}
\usepackage{ifxetex,ifluatex}
\ifnum 0\ifxetex 1\fi\ifluatex 1\fi=0 % if pdftex
  \usepackage[T1]{fontenc}
  \usepackage[utf8]{inputenc}
  \usepackage{textcomp} % provide euro and other symbols
\else % if luatex or xetex
  \usepackage{unicode-math}
  \defaultfontfeatures{Scale=MatchLowercase}
  \defaultfontfeatures[\rmfamily]{Ligatures=TeX,Scale=1}
\fi
% Use upquote if available, for straight quotes in verbatim environments
\IfFileExists{upquote.sty}{\usepackage{upquote}}{}
\IfFileExists{microtype.sty}{% use microtype if available
  \usepackage[]{microtype}
  \UseMicrotypeSet[protrusion]{basicmath} % disable protrusion for tt fonts
}{}
\makeatletter
\@ifundefined{KOMAClassName}{% if non-KOMA class
  \IfFileExists{parskip.sty}{%
    \usepackage{parskip}
  }{% else
    \setlength{\parindent}{0pt}
    \setlength{\parskip}{6pt plus 2pt minus 1pt}}
}{% if KOMA class
  \KOMAoptions{parskip=half}}
\makeatother
\usepackage{xcolor}
\IfFileExists{xurl.sty}{\usepackage{xurl}}{} % add URL line breaks if available
\IfFileExists{bookmark.sty}{\usepackage{bookmark}}{\usepackage{hyperref}}
\hypersetup{
  pdftitle={Simple Trial Report},
  hidelinks,
  pdfcreator={LaTeX via pandoc}}
\urlstyle{same} % disable monospaced font for URLs
\usepackage[margin=1in]{geometry}
\usepackage{graphicx}
\makeatletter
\def\maxwidth{\ifdim\Gin@nat@width>\linewidth\linewidth\else\Gin@nat@width\fi}
\def\maxheight{\ifdim\Gin@nat@height>\textheight\textheight\else\Gin@nat@height\fi}
\makeatother
% Scale images if necessary, so that they will not overflow the page
% margins by default, and it is still possible to overwrite the defaults
% using explicit options in \includegraphics[width, height, ...]{}
\setkeys{Gin}{width=\maxwidth,height=\maxheight,keepaspectratio}
% Set default figure placement to htbp
\makeatletter
\def\fps@figure{htbp}
\makeatother
\setlength{\emergencystretch}{3em} % prevent overfull lines

\setcounter{secnumdepth}{-\maxdimen} % remove section numbering

\title{Simple Trial Report}
\author{}
\date{\vspace{-2.5em}}

\begin{document}
\maketitle

\hypertarget{table-1}{%
\section{Table 1}\label{table-1}}

\includegraphics[width=4.75in,height=5.84in,keepaspectratio]{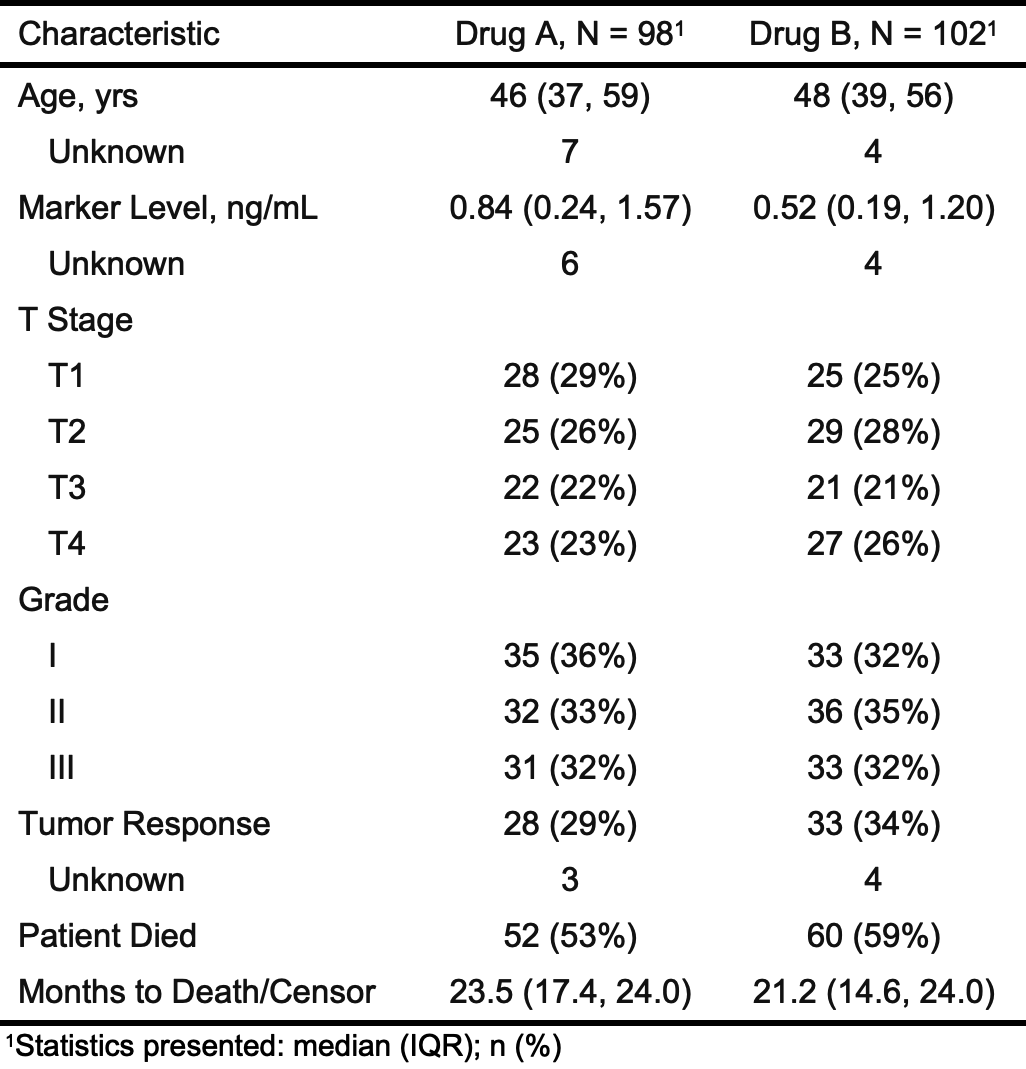}

\hypertarget{survival-plots}{%
\section{Survival Plots}\label{survival-plots}}

\hypertarget{overall}{%
\subsection{Overall}\label{overall}}

\includegraphics{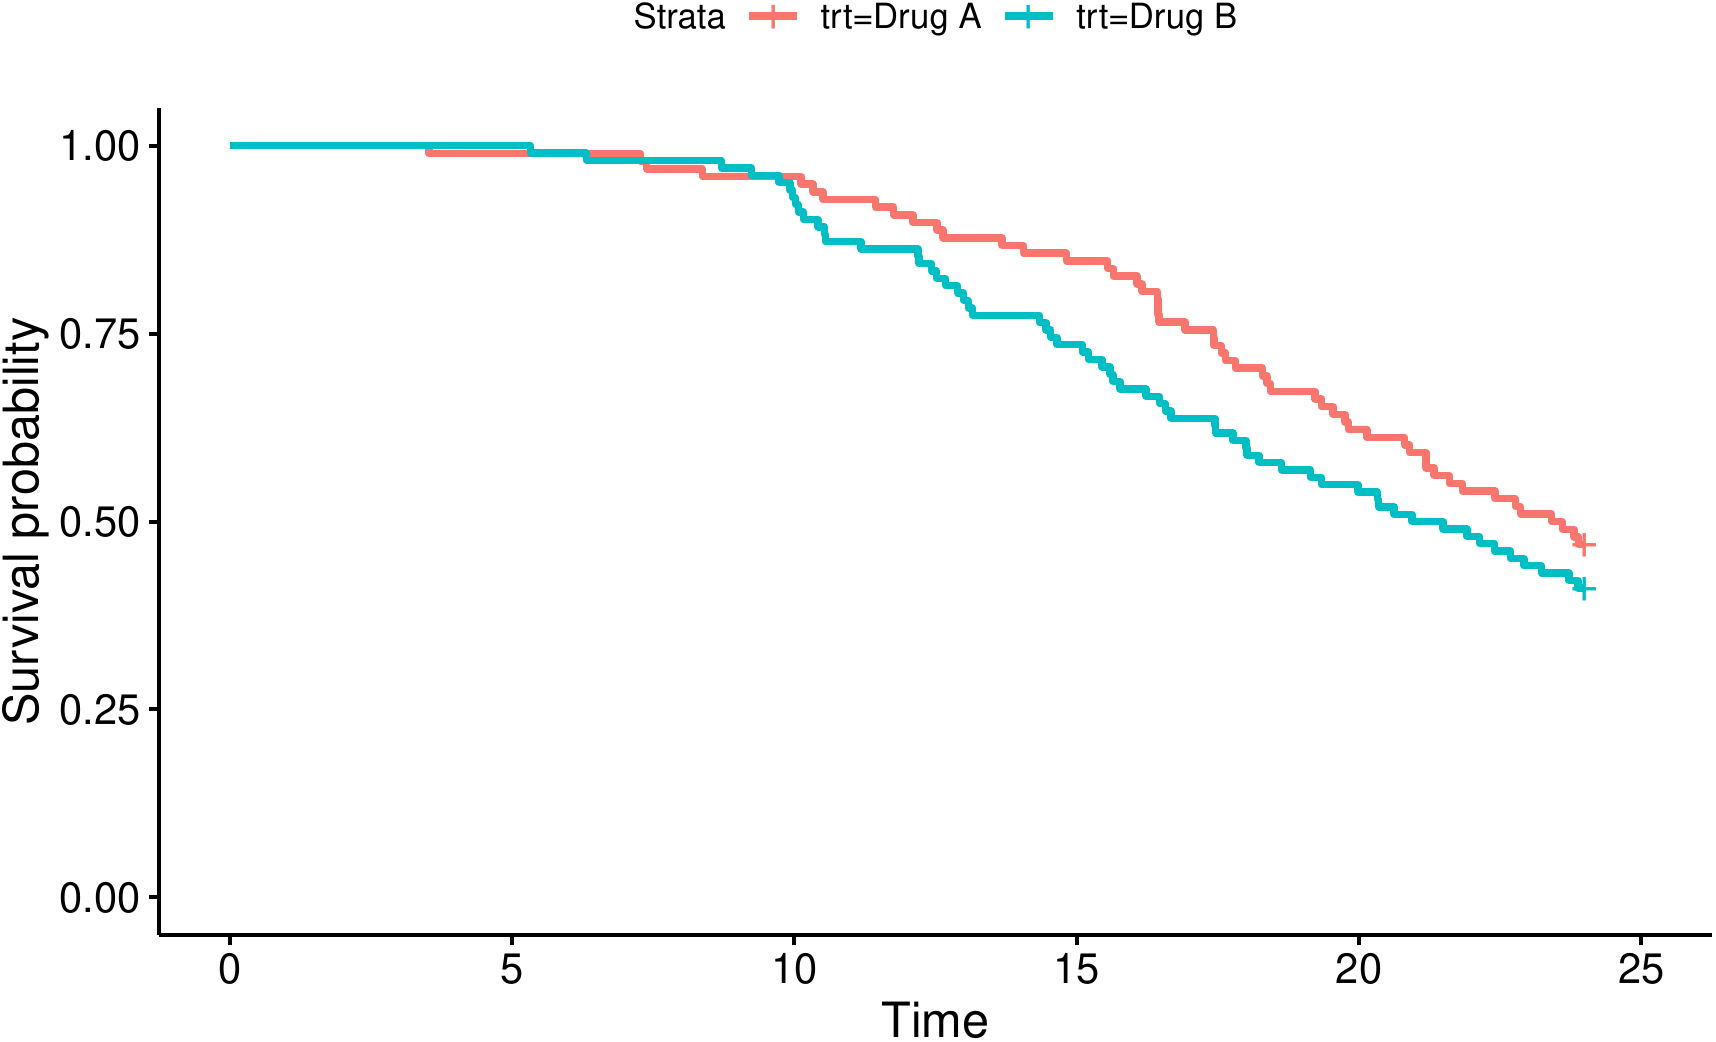}

\hypertarget{stage}{%
\subsection{Stage}\label{stage}}

\includegraphics{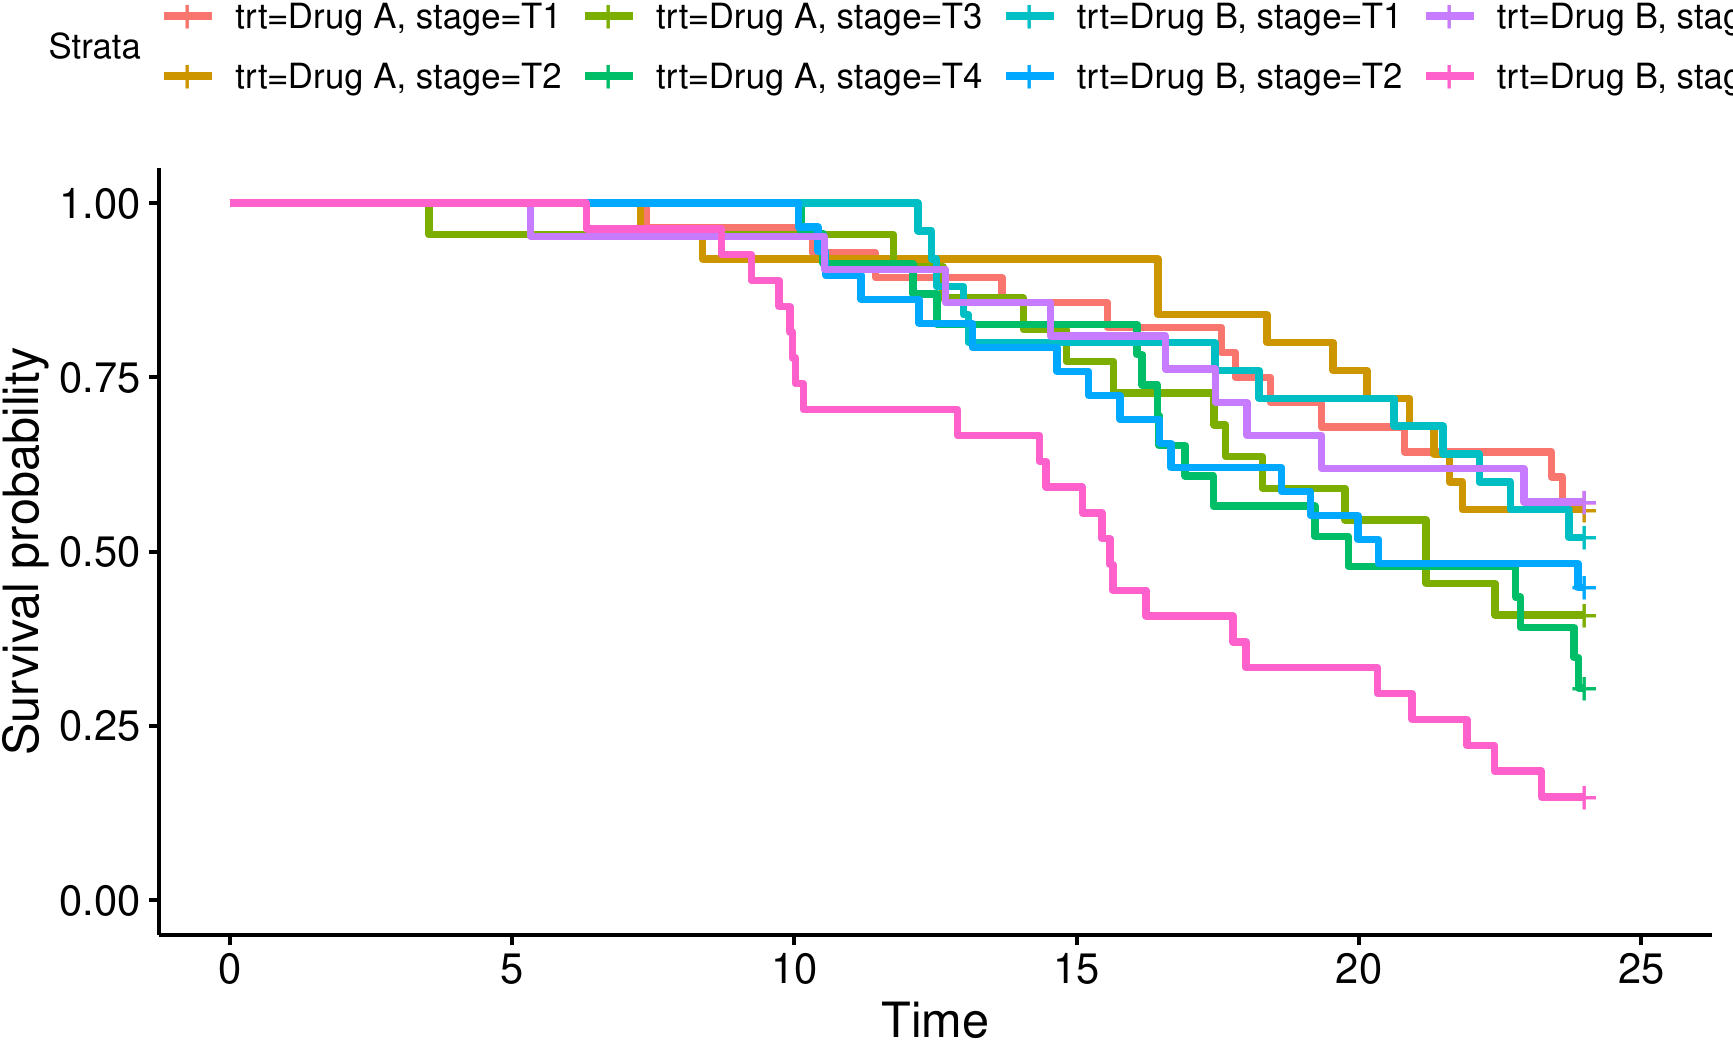}

\hypertarget{grade}{%
\subsection{Grade}\label{grade}}

\includegraphics{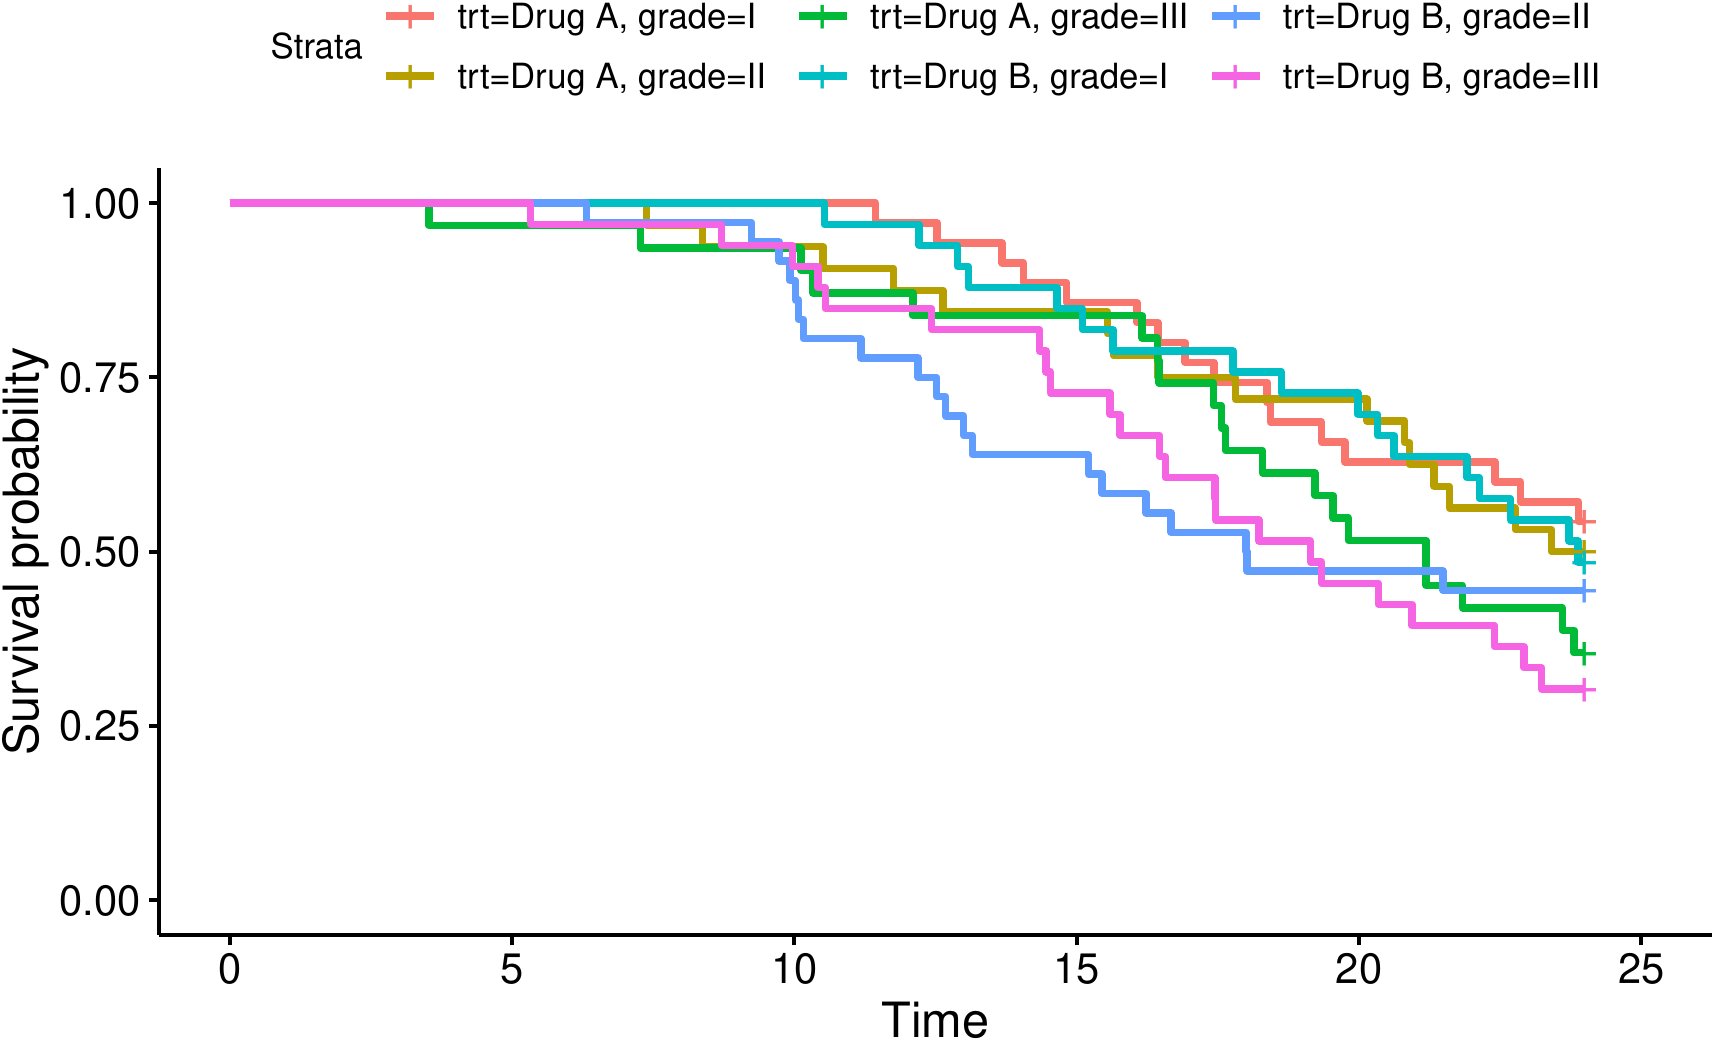}

\end{document}
